# Supplementary material for: Quantum-continuum simulation of underpotential deposition at electrified metal-solution interfaces
Source: arXiv:1701.01738 ancillary file (2017-01-06)
Supplement: Supplementary file 1 [file supplemental_information.pdf]

# Supplementary information for "Quantum–continuum simulation of underpotential deposition at electrified metal–solution interfaces"

Stephen E. Weitzner[1] and Ismaila Dabo[1]

[1]*Department of Materials Science and Engineering, Materials Research Institute, and Penn State Institutes of Energy and the Environment, The Pennsylvania State University, University Park, PA 16802, USA*

## NOTE 1. WORK FUNCTION CALCULATIONS

The work function data used to prepare Fig. 1 in the article is tabulated below in Table S.1. The work functions were computed with the PW code of QUANTUM-ESPRESSO. The ionic cores were represented with nonlinear core-corrected ultrasoft pseudopotentials. The exchange-correlation energy is modeled within the generalized gradient approximation using the parameterization proposed by Perdew, Burke, and Ernzerhof (PBE). The kinetic energy cutoff was set to 40 Ry and the charge density cutoff was set to 400 Ry after confirming the interatomic forces and total energies were converged within several meV/Å and a few tens of meV per cell, respectively. The Brillouin zone was sampled with a shifted $4 \times 4 \times 1$ Monkhorst–Pack grid and the electronic occupations were smoothed with 0.02 Ry of Marzari–Vanderbilt cold smearing. Each slab consisted of 17 to 18 layers, and was centered in the supercell with 10 Å of vacuum separating the periodically repeated slabs. The potential was corrected for periodic boundary artifacts using the generalized electrostatic solvers that have been implemented in the ENVIRON module referenced in the main body of the article. The top three layers on each side of the slab were allowed to relax, while the interior layers were fixed. The work function was taken to be the negative of the Fermi energy, which was aligned to a vacuum reference set to zero at the edge of the supercell, far away from the surface.

TABLE I: Theoretical single crystal work function data computed for Figure 1.

| Element | Surface orientation | Number of layers | Work function (eV) |
|---|---|---|---|
| Ag | 100 | 17 | 4.32 |
| | 111 | 17 | 4.43 |
| Au | 100 | 17 | 5.23 |
| | 111 | 17 | 5.18 |
| Bi | 0001 | 18 | 4.07 |
| Cd | 0001 | 17 | 3.94 |
| Cu | 100 | 17 | 4.65 |
| | 111 | 17 | 4.75 |
| Hg | 0001 | 17 | 4.21 |
| Pb | 100 | 17 | 3.78 |
| | 111 | 17 | 3.75 |
| Pt | 100 | 17 | 5.72 |
| | 111 | 17 | 5.71 |
| Tl | 0001 | 17 | 3.52 |
| Zn | 0001 | 18 | 4.23 |

## NOTE 2. DERIVING AN ANALYTICAL EXPRESSION FOR THE UNDERPOTENTIAL SHIFT

The underpotential shift $\Delta\Phi_{\mathrm{upd}} = \Phi_{\mathrm{S/M|M^{z+}}} - \Phi_{\mathrm{M|M^{z+}}}$ is characterized by the voltage at which an underpotentially deposited metal M desorbs from a nobler metal surface S compared to the reduction potential of M. This voltage shift can be understood in terms of the difference in chemical potential of M on the noble metal S and M on itself. Employing the model developed in the accompanying article, we show here how the underpotential shift can be computed analytically for a gold (100) surface with a coverage $\theta$ of copper adatoms. Below is a summary of the steps taken to prepare Fig. 3a in the main body of the article which is a contour plot of $\Delta\Phi_{\mathrm{upd}}$ for a half-covered gold (100) surface ($\theta = 0.5$) as a function of the double layer capacitance $C_{\mathrm{dl}}$ and the chemical potential of the hydrated copper ion $\mu_{\mathrm{Cu^{2+}}}$.

To begin, we consider Eq. 4 from the article, $\Delta\mu(N,\Phi) = \mu_{\mathrm{Cu}}(N,\Phi) - (\mu_{\mathrm{Cu^{2+}}} - 2e_0\Phi)$, which describes the energy required to add a copper atom from solution to the gold surface cell with $N$ copper adatoms. The cost to add a copper atom at an arbitrary coverage $\theta$ is then given by the linear interpolation (Eq. 10)

$$\Delta\mu(\theta,\Phi) = \frac{\Delta\mu(N=1,\Phi) + \Delta\mu(N=4,\Phi)}{2} + (2\theta - 1)\,\frac{\Delta\mu(N=4,\Phi) - \Delta\mu(N=1,\Phi)}{2}. \tag{S.1}$$

Setting $\theta = 0.5$ and considering the case when the system is at equilibrium ($\Delta\mu(\theta = 0.5, \Phi_{\mathrm{upd}}) = 0$), we obtain

$$\mu(N=1,\Phi_{\mathrm{upd}}) + \mu(N=4,\Phi_{\mathrm{upd}}) - 2(\mu_{\mathrm{Cu^{2+}}} - 2e_0\Phi_{\mathrm{upd}}) = 0. \tag{S.2}$$

Combining Eq. 7 and Eq. 8 from the article, the chemical potential of copper for the surface cell with $N$ copper adatoms and at a potential $\Phi$ can be expressed as:

$$\mu_{\mathrm{Cu}}(N,\Phi) = F_0(N) - F_0(N-1) + C_{\mathrm{dl}}\big(\Phi_0(N) - \Phi_0(N-1)\big)\left(\Phi - \frac{1}{2}\big(\Phi_0(N) + \Phi_0(N-1)\big)\right). \tag{S.3}$$

Inserting Eq. S.3 into Eq. S.2 and after performing some simple algebra, it can be shown that

$$\Phi_{\mathrm{upd}}(\mu_{\mathrm{Cu^{2+}}}, C_{\mathrm{dl}}) = \frac{F_0(0) - F_0(1) + F_0(3) - F_0(4) + 0.5(\Phi_0(1)^2 - \Phi_0(0)^2 + \Phi_0(4)^2 - \Phi_0(3)^2)C_{\mathrm{dl}} + 2\mu_{\mathrm{Cu^{2+}}}}{4e_0 + (\Phi_0(1) - \Phi_0(0) + \Phi_0(4) - \Phi_0(3))C_{\mathrm{dl}}} \tag{S.4}$$

where we explicitly define the dependence of the potential $\Phi_{\mathrm{upd}}$ on the interfacial capacitance and the chemical potential of the copper ions in solution, which is defined to be $\mu_{\mathrm{Cu^{2+}}} = \mu^{\circ}_{\mathrm{Cu^{2+}}} + k_{\mathrm{B}}T \ln a_{\mathrm{Cu^{2+}}}$. In order to compute the underpotential shift, we must reference the potential $\Phi_{\mathrm{upd}}$ to the reduction potential $\Phi_{\mathrm{Cu|Cu^{2+}}}$. However, since we have considered the chemical potential of copper ions under non-standard conditions, we must employ the Nernst equation to determine the non-standard reduction potential of copper

$$\Phi_{\mathrm{Cu|Cu^{2+}}} = \Phi^{\circ}_{\mathrm{Cu|Cu^{2+}}} + \frac{k_{\mathrm{B}}T}{2e_0}\ln a_{\mathrm{Cu^{2+}}}, \tag{S.5}$$

where $\Phi^{\circ}_{\mathrm{Cu|Cu^{2+}}} = 0.34$ V/SHE is the literature value of the standard reduction potential. This enables us to directly calculate $\Delta\Phi_{\mathrm{upd}}(\mu_{\mathrm{Cu^{2+}}}, C_{\mathrm{dl}}) = \Phi_{\mathrm{upd}}(\mu_{\mathrm{Cu^{2+}}}, C_{\mathrm{dl}}) - \Phi_{\mathrm{Cu|Cu^{2+}}}$.

## NOTE 3. COPPER ADLAYER CONFIGURATIONS

The four adsorption sites of the (2×2) surface cell were filled with different occupations of copper adatoms leading to a total of six unique surface structures. In the case of the half-covered surface, the copper adlayer can take on two different configurations within the surface cell, as shown below in Fig. S.1.

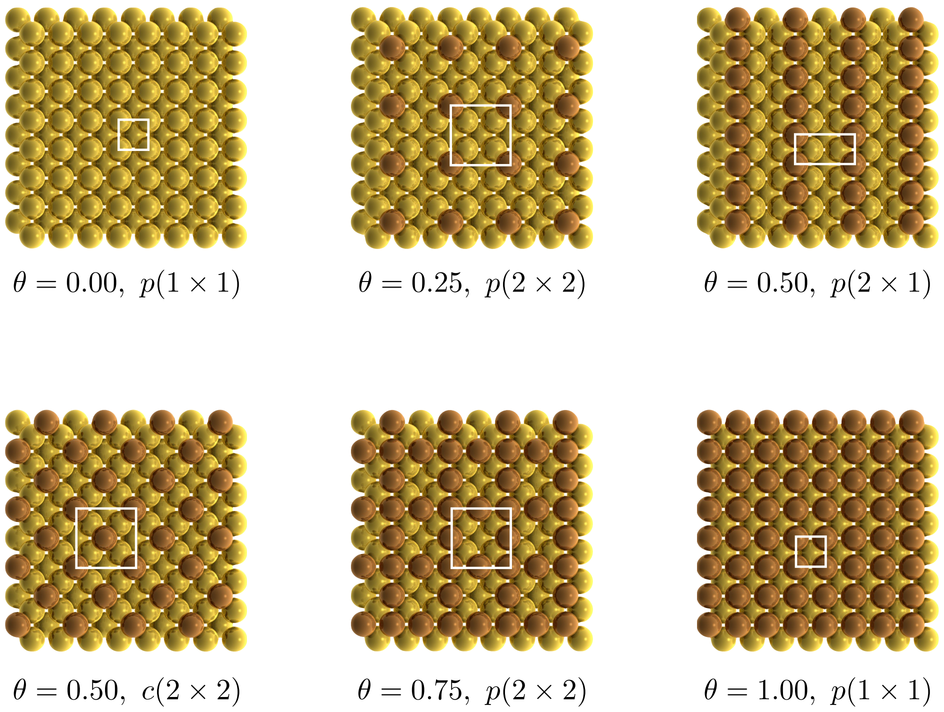


FIG. S.1: The set of surface configurations used in this work to compute the voltage-coverage curves. The white rectangles represent the adsorbate unit cell indicated below each surface.
